# Supplementary material for: Intermediate Service Facility Planning in a Stochastic and Competitive Market: Incorporating Agent-infrastructure Interactions over Networks
Source: arXiv:2304.00669 source file (2023-04-03)
Supplement: Supplementary file 1 [file app_derivatives.tex]

% jd 2015-05-22 23:30
\chapter{Calculation of ${\partial \rho_{k'}}/{\partial g_i^j}$}\label{app: part_rho_part_g}

${\partial \rho_{k'}}/{\partial g_i^j}$ can be computed from the ISO's optimization problem (\ref{DP_ISO_nn_t}), where $\boldsymbol{\rho}$ is the dual variables of constraint (\ref{DP_ISO_fc2}) and $\boldsymbol{g}$ is parameters. ${\partial \rho_{k'}}/{\partial g_i^j}$ is essentially the derivative of dual variables with respect to right-hand side constants. We use the standard  notations for convex optimization with linear constraints:

\begin{subequations}\label{eq:stan_opti_nota}
\begin{alignat}{2}
\min_{\boldsymbol{x}}
&\phantom{===} \hspace{0.5cm} &&\phantom{=}f(\boldsymbol{x})   \label{stan_opti_of}\\
 \text{s.t.}
&\phantom{===} (\boldsymbol{\lambda}) &&\phantom{=}A\boldsymbol{x}=\boldsymbol{b}\label{stan_opti_cons}
\end{alignat}
\end{subequations}
 
\noindent where $f(\boldsymbol{x})$ is a convex function and $\boldsymbol{x} \in \mathbb{R}^n, \boldsymbol{\lambda}, \boldsymbol{b} \in \mathbb{R}^m$, to illustrate the calculating process and our goal is to calculate the Jacobian matrix $J_{\boldsymbol{\lambda}}(\boldsymbol{b})$.

Lagrangian of problem (\ref{eq:stan_opti_nota}) is $\mathcal{L} = f(\boldsymbol{x}) - \boldsymbol{\lambda}^{T}(A\boldsymbol{x}-\boldsymbol{b})$. The optimality conditions of problem (\ref{eq:stan_opti_nota}) is:

\begin{subequations}\label{eq:stan_opti_opti_cond}
\begin{align}
\nabla f(\boldsymbol{x}) - A^T\boldsymbol{\lambda} &= \boldsymbol{0}\label{stan_opti_opti_cond1}\\
A\boldsymbol{x}-\boldsymbol{b} &= \boldsymbol{0}\label{stan_opti_opti_cond2}
\end{align}
\end{subequations}

Take implicit derivatives of equations (\ref{eq:stan_opti_opti_cond}) with respect to $\boldsymbol{b}$ :

\begin{subequations}\label{eq:stan_opti_opti_cond_impl_deri}
\begin{align}
\nabla^2_{\boldsymbol{x}} f(\boldsymbol{x^{\ast}}(\boldsymbol{b})) J_{\boldsymbol{x}}(\boldsymbol{b}) - A^T J_{\boldsymbol{\lambda}}(\boldsymbol{b}) &= \boldsymbol{0}\label{stan_opti_opti_cond1_impl_deri}\\
AJ_{\boldsymbol{x}}(\boldsymbol{b})-\boldsymbol{I} &= \boldsymbol{0}\label{stan_opti_opti_cond2_impl_deri}
\end{align}
\end{subequations}

The unknown variables in equations (\ref{eq:stan_opti_opti_cond_impl_deri}) are two Jacobian matrices, $J_{\boldsymbol{x}}(\boldsymbol{b})$ and $J_{\boldsymbol{\lambda}}(\boldsymbol{b})$. The total number of equations is equal to the total number of variables in equations (\ref{eq:stan_opti_opti_cond_impl_deri}), which is $nm+m^2$. Therefore, in most cases, $J_{\boldsymbol{\lambda}}(\boldsymbol{b})$ can be calculated given $\boldsymbol{b}$. Numerically, one can take an initial guess of $\boldsymbol{b}$ based on historical data and then solve equations (\ref{eq:stan_opti_opti_cond_impl_deri}) and Algorithm \ref{alg: ph_trans} iteratively until $J_{\boldsymbol{\lambda}}(\boldsymbol{b})$ converged.
