# Supplementary material for: Intermediate Service Facility Planning in a Stochastic and Competitive Market: Incorporating Agent-infrastructure Interactions over Networks
Source: arXiv:2304.00669 source file (2023-04-03)
Supplement: Supplementary file 2 [file app_flow.tex]

\chapter{Small Example Illustrating Flow Conservation Constraint (\ref{DP_ISO_alf}) $\sim$ (\ref{DP_ISO_fc3})}\label{App:flow_exam}

\subsection*{Network Structure}
 \begin{figure}[htbp]
\begin{center}
    \includegraphics[width=0.4\textwidth]{./Figures/Energy/6node_network_structure.pdf}
\caption{Small Example Structure}
\label{fig:smal_exam_stru}
\end{center}
\end{figure}

\subsection*{OD and Path Information}
 \begin{table}[htbp]
 \caption{Small Example Structure}
 \vspace{-0.5cm}
\begin{center}
    \includegraphics[width=0.7\textwidth]{./Figures/Energy/od_path.pdf}
\label{fig:od_path}
\end{center}
\end{table}
\pagebreak
\subsection*{Network Flow}
 \begin{figure}[h]
\begin{center}
    \includegraphics[width=0.9\textwidth]{./Figures/Energy/network_flow.pdf}
\label{fig:netw_flow}
\caption*{}
\end{center}
\end{figure}
\vspace{-2cm}
\subsection*{Incidence Matrix}
 \begin{figure}[h]
\begin{center}
    \includegraphics[width=0.9\textwidth]{./Figures/Energy/incidence_matrix.pdf}
\label{fig:inci_matr}
\caption*{}
\end{center}
\end{figure}
